# Supplementary material for: Low-Depth Parallel Algorithms for the Binary-Forking Model without Atomics
Source: arXiv:2008.13292 source file (2020-09-02)
Supplement: Supplementary file 1 [file mm-appendix.tex]

\section{Appendix}

\begin{figure*}
\begin{minipage}{0.56\textwidth}
\begin{mycolorbox}{\textsc{MM}$(X, U, V)$ \xcomment In-place 2-D}
\begin{minipage}{0.99\textwidth}
{\codesize
\algotopspace{}
\noindent
\begin{enumerate}
\setlength{\itemindent}{-2em}

\vsitem \xif $X$ is a small matrix \xthen $\textsc{MM\textrm{-}Loop}(X, U, V)$
\vsitem \xelse
\vsitem \T \xparallel \textsc{MM}$(X_{11}, U_{11}, V_{11})$, \textsc{MM}$(X_{12}, U_{11}, V_{12})$
\vsitem[] \xblankparallel \textsc{MM}$(X_{21}, U_{21}, V_{11})$, \textsc{MM}$(X_{22}, U_{21}, V_{12})$
\vsitem \T \xparallel \textsc{MM}$(X_{11}, U_{12}, V_{21})$, \textsc{MM}$(X_{12}, U_{12}, V_{22})$
\vsitem[] \xblankparallel \textsc{MM}$(X_{21}, U_{22}, V_{21})$, \textsc{MM}$(X_{22}, U_{22}, V_{22})$						

\algobottomspace{}
\end{enumerate}
}
\end{minipage}
\end{mycolorbox}
\vspace{-0.2cm}
\begin{mycolorbox}{\textsc{MM-HD}$(X, U, V, r)$ \xcomment Hybrid dynamic 2.5-D}
\begin{minipage}{0.99\textwidth}
{\codesize
\vspace{-0.25cm}
\algorequire $\Th{rn^2}$ space, $rn^2$ processors

\noindent
\begin{enumerate}
\setlength{\itemindent}{-2em}

\vsitem \textsc{MM-HD$'$}$(X, U, V, 0, r - 1)$ \xcomment Uses $r \in [1, n]$ planes

\algobottomspace{}
\end{enumerate}
}
\end{minipage}
\end{mycolorbox}
\vspace{-0.2cm}
\begin{mycolorbox}{\textsc{MM-OPT}$(X^{[0 .. r - 1]}, U, V)$ \xcomment Hybrid static 2.5-D}
\begin{minipage}{0.99\textwidth}
{\codesize
\vspace{-0.25cm}
\algorequire $\Th{rn^2}$ space, $rn^2$ processors

\noindent
\begin{enumerate}
\setlength{\itemindent}{-2em}

\vsitem Allocate $r \in [1, n]$ planes $X^{[0 .. r - 1]}$ all at once
\vsitem \textsc{MM-OPT$'$}$(X^{[0 .. r - 1]}, U, V)$ \xcomment Uses $r \in [1, n]$ planes
\vsitem \textsc{MM-ReduceR}$(X^{[0..r - 1]}, n, n)$

\algobottomspace{}
\end{enumerate}
}
\end{minipage}
\end{mycolorbox}
\vspace{-0.2cm}
\begin{mycolorbox}{\textsc{MM-ND}$(X, U, V, n)$ \xcomment Full not-in-place dynamic 3-D}
\begin{minipage}{0.99\textwidth}
{\codesize
\vspace{-0.25cm}
\algorequire $\Th{rn^2}$ space, $n^3$ processors

\noindent
\begin{enumerate}
\setlength{\itemindent}{-2em}

\vsitem \textsc{MM-HD$'$}$(X, U, V, 0, n - 1)$ \xcomment Uses $n$ planes

\algobottomspace{}
\end{enumerate}
}
\end{minipage}
\end{mycolorbox}
\vspace{-0.2cm}
\begin{mycolorbox}{\textsc{MM\textrm{-}NS}$(X^{[0 .. n - 1]}, U, V)$ \xcomment Full not-in-place static 3-D}
\begin{minipage}{0.99\textwidth}
{\codesize
\vspace{-0.25cm}
\algorequire $\Th{n^3}$ space, $n^3$ processors

\noindent
\begin{enumerate}
\setlength{\itemindent}{-2em}

\vsitem Allocate $n$ planes $X^{[0 .. n - 1]}$ all at once
\vsitem \textsc{MM-OPT$'$}$(X^{[0 .. n - 1]}, U, V)$ \xcomment Uses $n$ planes
\vsitem \textsc{MM-ReduceR}$(X^{[0..n - 1]}, n, n)$

\algobottomspace{}
\end{enumerate}
}
\end{minipage}
\end{mycolorbox}
\vspace{-0.2cm}
\begin{mycolorbox}{\textsc{MM-Tradeoff}$(X, U, V, p, E_p(n))$ \xcomment Trade-off}
\begin{minipage}{0.99\textwidth}
{\codesize
\vspace{-0.25cm}
\algorequire Extra space $E_p(n) = \Oh{ p \log n }$
%\algotopspace{}
\noindent
\begin{enumerate}
\setlength{\itemindent}{-2em}

\vsitem \xif $p \in [1, n^2]$ \xthen Use 2-D \textsc{MM} \xcomment 1 plane
\vsitem \xelseif $p \in ((r-1) n^2, rn^2]$ where $r \in [2, n]$ \xthen
\vsitem \T Use 2.5-D \textsc{MM-OPT} with $r$ planes \xcomment $r$ planes 
\algobottomspace{}
\end{enumerate}
}
\end{minipage}
\end{mycolorbox}
\end{minipage}
\begin{minipage}{0.65\textwidth}
\begin{mycolorbox}{\textsc{MM-HD$'$}$(X, U, V, \ell, h)$}
\begin{minipage}{0.99\textwidth}
{\codesize
\algotopspace{}
\noindent
\begin{enumerate}
\setlength{\itemindent}{-2em}

\vsitem \xif $\ell = h$ \xthen $\textsc{MM}(X, U, V)$ \xcomment Single plane
\vsitem \xelse \xcomment Multiple planes
\vsitem \T $m \gets ( \ell + h ) / 2$
\vsitem \T Allocate auxiliary matrix $Y$ at run time with size that as $X$
\vsitem \T \xpar \textsc{MM-HD$'$}$(X_{11}, U_{11}, V_{11}, \ell, m)$, \textsc{MM-HD$'$}$(X_{12}, U_{11}, V_{12}, \ell, m)$
\vsitem[] \xblankpar \textsc{MM-HD$'$}$(X_{21}, U_{21}, V_{11}, \ell, m)$, \textsc{MM-HD$'$}$(X_{22}, U_{21}, V_{12}, \ell, m)$,

\vsitem[] \xblankpar \textsc{MM-HD$'$}$(Y_{11}, U_{12}, V_{21}, m + 1, h)$, \textsc{MM-HD$'$}$(Y_{12}, U_{12}, V_{22}, m + 1, h)$

\vsitem[] \xblankpar \textsc{MM-HD$'$}$(Y_{21}, U_{22}, V_{21}, m + 1, h)$, \textsc{MM-HD$'$}$(Y_{22}, U_{22}, V_{22}, m + 1, h)$						

\vsitem \T \textsc{MM-Reduce2}$(X, Y, n)$
\vsitem \T Deallocate auxiliary matrix $Y$
\algobottomspace{}
\end{enumerate}
}
\end{minipage}
\end{mycolorbox}
\vspace{-0.2cm}
\begin{mycolorbox}{\textsc{MM-Reduce2}$(X, Y, n)$ \xcomment $X \gets X + Y$}
\begin{minipage}{0.99\textwidth}
{\codesize
\algotopspace{}
\noindent
\begin{enumerate}
\setlength{\itemindent}{-2em}

\vsitem \xparallelfor $i \gets 1$ \xto $n$ \xdo 
\vsitem \T \xparallelfor $J \gets 1$ \xto $\ceil{n/B}$ \xdo \xcomment $B =$ data block size
\vsitem \T \T $X[i, J\text{th data block}] \gets X[i, J\text{th data block}] + Y[i, J\text{th data block}]$

\algobottomspace{}
\end{enumerate}
}
\end{minipage}
\end{mycolorbox}
\vspace{-0.2cm}
\begin{mycolorbox}{\textsc{MM-OPT$'$}$(X^{[\ell .. h]}, U, V)$}
\begin{minipage}{0.99\textwidth}
{\codesize
\algotopspace{}
\noindent
\begin{enumerate}
\setlength{\itemindent}{-2em}

\vsitem \xif $\ell = h$ \xthen $\textsc{MM}(X^{[\ell]}, U, V)$ \xcomment Single plane
\vsitem \xelse \xcomment Multiple planes
\vsitem \T $m \gets ( \ell + h ) / 2$
\vsitem \T \xpar \textsc{MM-OPT$'$}$(X_{11}^{[\ell .. m]}, U_{11}, V_{11})$, \textsc{MM-OPT$'$}$(X_{12}^{[\ell .. m]}, U_{11}, V_{12})$
\vsitem[] \xblankpar \textsc{MM-OPT$'$}$(X_{21}^{[\ell .. m]}, U_{21}, V_{11})$, \textsc{MM-OPT$'$}$(X_{22}^{[\ell .. m]}, U_{21}, V_{12})$
\vsitem[] \xblankpar \textsc{MM-OPT$'$}$(X_{11}^{[m + 1 .. h]}, U_{12}, V_{21})$, \textsc{MM-OPT$'$}$(X_{12}^{[m + 1 .. h]}, U_{12}, V_{22})$
\vsitem[] \xblankpar \textsc{MM-OPT$'$}$(X_{21}^{[m + 1 .. h]}, U_{22}, V_{21})$, \textsc{MM-OPT$'$}$(X_{22}^{[m + 1 .. h]}, U_{22}, V_{22})$						
\algobottomspace{}
\end{enumerate}
}
\end{minipage}
\end{mycolorbox}
\vspace{-0.2cm}
\begin{mycolorbox}{\textsc{MM-ReduceR}$(X^{[0..r - 1]}_{a \times b}, a, b)$ \xcomment $X^{[0]} \gets X^{[0]} + \cdots + X^{[r - 1]}$}
\begin{minipage}{0.99\textwidth}
{\codesize
\algotopspace{}
\noindent
\begin{enumerate}
\setlength{\itemindent}{-2em}

\vsitem \xparallelfor $i \gets 1$ \xto $a$ \xdo 
\vsitem \T \xparallelfor $J \gets 1$ \xto $\ceil{b/B}$ \xdo \xcomment $B =$ data block size
\vsitem \T \T local \xreducer $sum[1..B]$ data block
\vsitem \T \T \xrfor $k \gets 0$ \xto $r - 1$ \xdo 
\vsitem \T \T \T $sum[1..B] \gets sum[1..B] + X^{[k]}[i, J\text{th data block}]$
\vsitem \T \T $X^{[0]}[i, J\text{th data block}] \gets sum[1..B]$ 

\algobottomspace{}
\end{enumerate}
}
\end{minipage}
\end{mycolorbox}
\end{minipage}
\vspace{-0.3cm}
\caption{In-place 2-D, full not-in-place 3-D, hybrid dynamic 2.5-D, and hybrid static 2.5-D algorithms for matrix multiplication. The algorithms are invoked with $U = A$, $V = B$, and $X$ being the total space available for the MM computation.}
\label{fig:matrixmultiplication}
\end{figure*}

\hide{
The naive cache-inefficient iterative algorithm is in-place and has a serial cache complexity of $\Th{n^3 / B + n^2}$ and a span of $\Th{n}$ or a parallelism of $\Th{n^2}$. The tiled cache-efficient cache-aware algorithm with tile size $\sqrt{M}$ has an optimal serial cache complexity of $\Th{n^3/(B \sqrt{M}) + n^2 / B + 1}$, assuming a tall cache i.e., $M = \Om{B^2}$, and has $\Th{n}$ span or $\Th{n^2}$ parallelism.
}

\para{\textsc{MM}: In-place 2-D Algorithm}
The in-place or 2-D algorithm introduced in \cite{BlumofeFrJoLeRa1996} as shown in Figure \ref{fig:matrixmultiplication} uses $E_p(n) = \Oh{p \log n}$ extra space (i.e., stack space for recursion) on a $p$-processor machine, where $p \in [1, n^2]$, and has a span of $\Th{n}$. From hereon, for simplicity, we do not consider the stack space for recursion when we compute the total space. The algorithm can be extended to rectangular matrices \cite{Prokop1999}. The in-place MM algorithm is shown in Figure \ref{fig:matrixmultiplication}. A standard iterative looping MM algorithm is invoked in the base case when a subtask size is a small constant. In general, the base cases of recursive divide-and-conquer algorithms are chosen as small constants such that the run time of reaching a base case through recursion is subsumed by the run time of computing the base case kernel.

\begin{lemma}[\highlighttitle{MM: In-place 2-D}]
	\label{lem:mm}
	The complexities of the MM algorithm are as follows: work, $T_1(n) = \Th{n^3}$; span, $T_{\infty}(n)=\Th{n}$; space, $S_{\infty}(n) = \Th{n^2}$; 
	% $E_p(n) = \Oh{p \log n}$, 
	and serial cache complexity, $Q_1(n) \allowbreak = \allowbreak \Th{n^3/(B \sqrt{M}) \allowbreak + n^3/M \allowbreak + n^2 / B \allowbreak + n + 1}$. 
\end{lemma}
\begin{proof}
The complexities follow from the following recurrences which can be derived from the recursive structure of the divide-and-conquer algorithm:\\

$T_1(n) = T_{\infty}(n) = S_{\infty}(n) = \Th{1} \qquad \text{if } n = 1,$

$T_1(n) = 8 T_1(n / 2) + \Th{1} \qquad \text{if } n > 1.$

$T_{\infty}(n) = 2 T_{\infty}(n / 2) + \Th{1} \qquad \text{if } n > 1.$

$S_{\infty}(n) = 4 S_{\infty}(n / 2) + \Th{1} \qquad \text{if } n > 1.$

% & E_p(n) = \Oh{ p E_1(n) } = \Oh{p \log n}.\\

$Q_1(n) = \begin{cases} \Th{n^2 / B + n} &\mbox{if } n^2 \le \alpha M,\\ 
Q_1(n / 2) + \Th{1}  & \mbox{if } n^2 > \alpha M. \end{cases}$
\hide{
\scalebox{0.9}
{
\centering
\begin{minipage}{0.49\textwidth}
\begin{align*}
& T_1(n) = T_{\infty}(n) = S_{\infty}(n) = \Th{1} \qquad \text{if } n = 1,\\
& T_1(n) = 8 T_1(n / 2) + \Th{1} \qquad \text{if } n > 1.\\
& T_{\infty}(n) = 2 T_{\infty}(n / 2) + \Th{1} \qquad \text{if } n > 1.\\
& S_{\infty}(n) = 4 S_{\infty}(n / 2) + \Th{1} \qquad \text{if } n > 1.\\
% & E_p(n) = \Oh{ p E_1(n) } = \Oh{p \log n}.\\
&Q_1(n) = \begin{cases} \Th{n^2 / B + n} &\mbox{if } n^2 \le \alpha M,\\ 
8 Q_1(n / 2) + \Th{1}  & \mbox{if } n^2 > \alpha M. \end{cases}
\end{align*}    
\end{minipage}
}\\
}
% hide ends
%
\end{proof}

MM can scale to a maximum number of $n^2$ processors. With full scalability (i.e., $p = n^2$), we might intuitively think that each processor computes all $n$ computations of a specific cell in the output $C$ matrix. However, this might not be the case depending on the \textit{parallel task scheduler} used (e.g.: randomized work stealing). This implies that the processors possibly can get an unequal number (i.e., $\ne n$) of basic operations (i.e., multiplication) to compute.

\para{MM-HD: Hybrid Dynamic 2.5-D Algorithm}
MM-HD hybrid 2.5-D algorithm with dynamic memory allocation is a generalization of the  dynamic memory MM algorithm presented in Chapter 27 of \cite{CormenLeRiSt2009}. The \textsc{MM-HD} algorithm is given in Figure \ref{fig:matrixmultiplication}.

\textsc{MM-HD} calls \textsc{MM-HD$'$}. The recursive function \textsc{MM-HD$'$} invokes eight child functions in a single parallel step. In each invocation of \textsc{MM-HD$'$}, an auxiliary matrix $Y$ is created at run time before invoking the child functions. After the execution of all child functions, the matrices $X$ and $Y$ are added using the function \textsc{MM-Reduce2} and the result is stored in $X$. Finally, we deallocate the dynamic memory for matrix $Y$.

Let's call a single $n \times n$ matrix as a \textit{plane}. We set the parameter $r$ in the range $[1, n]$ to make sure that we use at most $r n^2$ total space (i.e., $r$ planes) and at most $r n^2$ \#processors. We use the variables $\ell$ and $h$ to make sure that we use at most $(h - \ell)$ auxiliary planes and at most $(h - \ell + 1)$ total planes in the corresponding divide-and-conquer function. The complexity of the algorithm is given in Theorem \ref{thm:mm-hd}.

\begin{theorem}[\highlighttitle{MM-HD: Hybrid dynamic 2.5-D}]
\label{thm:mm-hd} MM-HD\\has a complexity of $T_1(n) = \Th{n^3}$, $S_{\infty}(n) =\Th{r n^2}$,\\ $T_{\infty}(n)=\Oh{n/r + \log r(2\log n - \log r + B)}$, and\\
$Q_1(n) = \left\{
\begin{array}{lr}
\Oh{ (n^3 / (B \sqrt{M}) + n^3 / M + r n^2 / B + r^2 n} & \text{if } f > r, \\
\Oh{ rn^2 / B + n f ( r + n/B + f ) } & \text{if } f \le r.
  \end{array}
\right\}$\\
where $f = (rn^2/M)^{1/3}$. 
\end{theorem}
\begin{proof}
When the input size parameter drops to $n / r$, we switch from executing \textsc{MM-HD$'$} to \textsc{MM}. Hence, in the following recurrences, when the problem size reaches the base case (i.e., when $r = 1$), the complexities are the same as the complexities from Lemma \ref{lem:mm}. Thus, we have\\

$T_1(n, r) = \begin{cases} \Th{n^3} &\mbox{if } r = 1, \\ 
8 T_1(n/2, r/2) + \Th{n^2}  & \mbox{if } r > 1. \end{cases}$

$T_{\infty}(n, r) = \begin{cases} \Th{n} &\mbox{if } r = 1, \\ 
T_{\infty}(n/2, r/2) + \Th{\log n + B}  & \mbox{if } r > 1. \end{cases}$

$S_{\infty}(n, r) \le \begin{cases} \Th{n^2} &\mbox{if } r = 1,\\
8 S_{\infty}(n/2, r/2) + \Th{1}  & \mbox{if } r > 1. \end{cases}$

$Q_1(n, r) = \begin{cases} Q_1^{A}(n, r) &\mbox{if } r < n/\sqrt{M}, \\ 
Q_1^{B}(n, r)  & \mbox{if } r \ge n/\sqrt{M}. \end{cases}$

$Q_1^{A}(n, r) = \begin{cases} \Oh{n^3 / (B\sqrt{M}) + n^3 / M + n^2 / B + n} &\mbox{if } r = 1, \\ 
8 Q_1^{A}(n/2, r/2) + \Oh{n^2 / B + n}  & \mbox{if } r > 1. \end{cases}$

$Q_1^{B}(n, r) = \begin{cases} \Oh{rn^2 / B + rn} &\mbox{if } r n^2 \le \alpha M, \\ 
8 Q_1^{B}(n/2, r/2) + \Oh{n^2 / B + n}  & \mbox{if } rn^2 > \alpha M. \end{cases}$

\hide{
\scalebox{0.9}
{
\centering
\begin{minipage}{0.49\textwidth}
\begin{align*}
&T_1(n, r) = \begin{cases} \Th{n^3} &\mbox{if } r = 1, \\ 
8 T_1(n/2, r/2) + \Th{n^2}  & \mbox{if } r > 1. \end{cases}\\
&T_{\infty}(n, r) = \begin{cases} \Th{n} &\mbox{if } r = 1, \\ 
T_{\infty}(n/2, r/2) + \Th{\log n + B}  & \mbox{if } r > 1. \end{cases}\\
&S_{\infty}(n, r) \le \begin{cases} \Th{n^2} &\mbox{if } r = 1,\\
8 S_{\infty}(n/2, r/2) + \Th{1}  & \mbox{if } r > 1. \end{cases}\\
&Q_1(n, r) = \begin{cases} Q_1^{A}(n, r) &\mbox{if } r < n/\sqrt{M}, \\ 
Q_1^{B}(n, r)  & \mbox{if } r \ge n/\sqrt{M}.
\end{cases}\\
&Q_1^{A}(n, r) = \begin{cases} \Oh{n^3 / (B\sqrt{M}) + n^3 / M + n^2 / B + n} &\mbox{if } r = 1, \\ 
8 Q_1^{A}(n/2, r/2) + \Oh{n^2 / B + n}  & \mbox{if } r > 1.
\end{cases}\\
&Q_1^{B}(n, r) = \begin{cases} \Oh{rn^2 / B + rn} &\mbox{if } r n^2 \le \alpha M, \\ 
8 Q_1^{B}(n/2, r/2) + \Oh{n^2 / B + n}  & \mbox{if } rn^2 > \alpha M.
\end{cases}
\end{align*}
\end{minipage}
}\\
}
% hide ends

We compute $Q_1$ using two cases: $[$Case $A.]$ In this case, a subproblem switches to the in-place algorithm before fitting in the cache i.e, $(n/r)^2 > M$ or $r < n/\sqrt{M}$. Recurrence $Q_1^{A}$ models this case. We get $Q_1^{A}(n, r) = \Oh{n^3/(B \sqrt{M}) + n^3/M + rn^2/B + r^2n}$. $[$Case $B.]$ In this case, a subproblem fits in the cache before switching to the in-place algorithm i.e, $(n/r)^2 \le M$ or $r \ge n/\sqrt{M}$. Recurrence $Q_1^{B}$ models this case. We get $Q_1^{B}(n, r) = \Oh{ \frac{rn^2}{B} + \frac{r^{4/3} n^{5/3}}{M^{1/3}} + \frac{r^{1/3}n^{8/3}}{BM^{1/3}} + \frac{r^{2/3}n^{7/3}}{M^{2/3}}}$.

For simplicity, we assume that we can allocate polynomial of $n$ memory dynamically in logarithmic time w.r.t $n$. The additive terms in $T_{\infty}$ and $Q_{1}$ recurrences are $\Th{\log n + B}$ and $\Oh{n^2 / B + n}$, respectively because they are the span and serial cache complexity of the \textsc{MM-Reduce2} function for $n \times n$ matrices. Note that reducing the span of \textsc{MM-Reduce2} to $\Th{\log n}$ negatively affects the cache performance as we cannot simultaneously achieve optimal cache performance and optimal span for \textsc{MM-Reduce2}.
\end{proof}

\highlighttitle{MM-HD: Hybrid dynamic 2.5-D}.
Theorem \ref{thm:mm-hd} details are below:
\begin{align*}
&Q_1^{A}(n, r) = 8 Q_1^{A}\left( \frac{n}{2}, \frac{r}{2} \right) + \left( \frac{n^2}{B} + n \right)\\
&= 8 \left( 8 Q_1^{A}\left( \frac{n}{2^2}, \frac{r}{2^2} \right) + \left( \frac{1}{B} \left( \frac{n}{2} \right)^2 + \frac{n}{2} \right) \right) + \left( \frac{n^2}{B} + n \right) \\
&\le 8^k Q_1^{A}\left( \frac{n}{2^k}, \frac{r}{2^k} \right) + \frac{2^k n^2}{B} + 4^k n\\
&= 8^{\log r} \cdot Q_1^{A} \left( \frac{n}{2^{\log r}}, \frac{r}{2^{\log r}} \right) + \frac{2^{\log r} n^2}{B} + 4^{\log r} n\\
&= r^3 \cdot Q_1^{A} \left( \frac{n}{r}, \frac{r}{r} \right) + \frac{r n^2}{B} + r^2 n \\
&= r^3 \Oh{ \frac{n^3}{r^3 B \sqrt{M}} + \frac{n^3}{r^3 M} + \frac{n^2}{r^2 B} + \frac{n}{r} } + \frac{r n^2}{B} + r^2 n \\
&= \Oh{ \frac{n^3}{B \sqrt{M}} + \frac{n^3}{M} + \frac{r n^2}{B} + r^2 n}
\end{align*}
\begin{align*}
&Q_1^{B}(n, r) = 8 Q_1^{B}\left( \frac{n}{2}, \frac{r}{2} \right) + \left( \frac{n^2}{B} + n \right) \le 8^k Q_1^{B}\left( \frac{n}{2^k}, \frac{r}{2^k} \right) + \frac{2^k n^2}{B} + 4^k n\\
&= 8^{k} \Oh{\frac{r}{2^{k}} \left( \frac{n}{2^{k}} \right)^2 \frac{1}{B} + \frac{r}{2^{k}} \frac{n}{2^{k}}  } + \frac{2^k n^2}{B} + 4^k n \qquad \left(\because \frac{rn^2}{8^{k}} = M \right)\\
&\le 8^{k} \Oh{\frac{M}{B} + \sqrt{M\frac{r}{2^{k}}}} + \frac{n^2}{B} \left( \frac{rn^2}{M} \right)^{1/3} + n \left( \frac{rn^2}{M} \right)^{2/3} \\
&= \frac{rn^2}{M} \Oh{\frac{M}{B} + \sqrt{M\frac{r}{(rn^2/M)^{1/3}}}} + \frac{r^{1/3}n^{8/3}}{BM^{1/3}} + \frac{r^{2/3}n^{7/3}}{M^{2/3}}\\
&= \Oh{ \frac{rn^2}{B} + \frac{r^{4/3} n^{5/3}}{M^{1/3}} + \frac{r^{1/3}n^{8/3}}{BM^{1/3}} + \frac{r^{2/3}n^{7/3}}{M^{2/3}}}\\
&= \Oh{ \frac{rn^2}{B} + n \left( \frac{rn^2}{M} \right)^{1/3} \left( r + \frac{n}{B} + \left( \frac{rn^2}{M} \right)^{1/3} \right) }
\end{align*}

\noindent
\highlighttitle{MM-OPT: Hybrid static 2.5-D}.
Theorem \ref{thm:MM-OPT} details are below:
\begin{align*}
&Q_1^{A}(n, r) = 8 Q_1^{A}\left( \frac{n}{2}, \frac{r}{2} \right) + 1 = 8 \left( 8 Q_1^{A}\left( \frac{n}{2^2}, \frac{r}{2^2} \right) + 1 \right) + 1 \\
&\le 8^{\log r} \left( Q_1^{A} \left( \frac{n}{2^{\log r}}, \frac{r}{2^{\log r}} \right) + 1 \right) = r^3 \left( Q_1^{A} \left( \frac{n}{r}, \frac{r}{r} \right) + 1 \right)\\
&= r^3 \Oh{ \frac{n^3}{r^3 B \sqrt{M}} + \frac{n^3}{r^3 M} + \frac{n^2}{r^2 B} + \frac{n}{r} + 1 }\\
&= \Oh{ \frac{n^3}{B \sqrt{M}} + \frac{n^3}{M} + \frac{r n^2}{B} + r^2 n + r^3 }
\end{align*}
\begin{align*}
&Q_1^{B}(n, r) = 8 Q_1^{B}\left( \frac{n}{2}, \frac{r}{2} \right) + 1 = 8 \left( 8 Q_1^{B}\left( \frac{n}{2^2}, \frac{r}{2^2} \right) + 1 \right) + 1 \\
&\le 8^{k} \left( Q_1^{B} \left( \frac{n}{2^{k}}, \frac{r}{2^{k}} \right) + 1 \right) = 8^{k} \Oh{\frac{r}{2^{k}} \left( \frac{n}{2^{k}} \right)^2 \frac{1}{B} + \frac{r}{2^{k}} \frac{n}{2^{k}}  + 1}\\
&\le 8^{k} \Oh{\frac{M}{B} + \sqrt{M\frac{r}{2^{k}}} + 1} \qquad \left(\because \frac{rn^2}{8^{k}} = M \right)\\
&= \frac{rn^2}{M} \Oh{\frac{M}{B} + \sqrt{M\frac{r}{(rn^2/M)^{1/3}}} + 1} = \Oh{ \frac{rn^2}{B} + \frac{r^{4/3} n^{5/3}}{M^{1/3}} + \frac{rn^2}{M}}\\
&= \Oh{ \frac{rn^2}{B} + \left( \frac{rn^2}{M} \right)^{1/3} \left( nr + \left( \frac{rn^2}{M} \right)^{2/3}  \right) }
\end{align*}

\hide{
\begin{theorem}
Suppose that the total space used by \textsc{MM-OPT} is $r n^2$ where $r$ is the number of planes used. Then to remain cache-optimal, the value of $r$ must satisfy the following:
$$
r \le \mbox{min}\Big(\frac{n}{M^{3/4}}, \frac{n}{M^{1/2}\log^{1/3}n}\Big).
$$
\end{theorem}
}

\para{\textsc{MM-ND/MM-NS}: Full Not-in-place 3-D Dynamic/Static Algorithm}
The MM-ND/MM-NS algorithms as shown in Figure \ref{fig:matrixmultiplication} with full scalability require a gigantic $\Th{n^3}$ total space and $n^3$ processors. MM-ND and MM-NS are obtained by setting $r = n$ in MM-ND and MM-NS, respectively, to achieve low spans of $\Th{\log^2 n}$ and $\Th{\log n}$, respectively.

\begin{lemma}[\highlighttitle{\textsc{MM-ND/MM-NS}: Full not-in-place dynamic or static 3-D}]
\label{lem:mmn}
\textsc{MM-ND} and \textsc{MM-NS} have a complexity of $T_1(n) = \Th{n^3}$,  $S_{\infty}(n) = \Th{n^3}$, $T_{\infty}^{\textsc{MM-ND}}(n)=\Th{\log n (\log n + B)}$,\\
$T_{\infty}^{\textsc{MM-NS}}(n)=\Th{\log n + B}$, and $Q_{1}(n) = \Oh{n^3/B + n^3/M^{1/3} + 1}$.
\end{lemma}
\begin{proof}
The complexities can be computed by simply substituting $r = n$ in Theorems \ref{thm:mm-hd} and \ref{thm:MM-OPT}. We can compute $Q_{n^3}(n)$ for randomized work-stealing scheduler by setting $p = n^3$ (full scalability) in the formula $Q_{p}(n) = \Oh{Q_1 + p T_{\infty} (M/B)}$.
\end{proof}

\begin{figure}
\begin{minipage}{0.5\textwidth}
\flushleft
\includegraphics[width=0.95\textwidth]{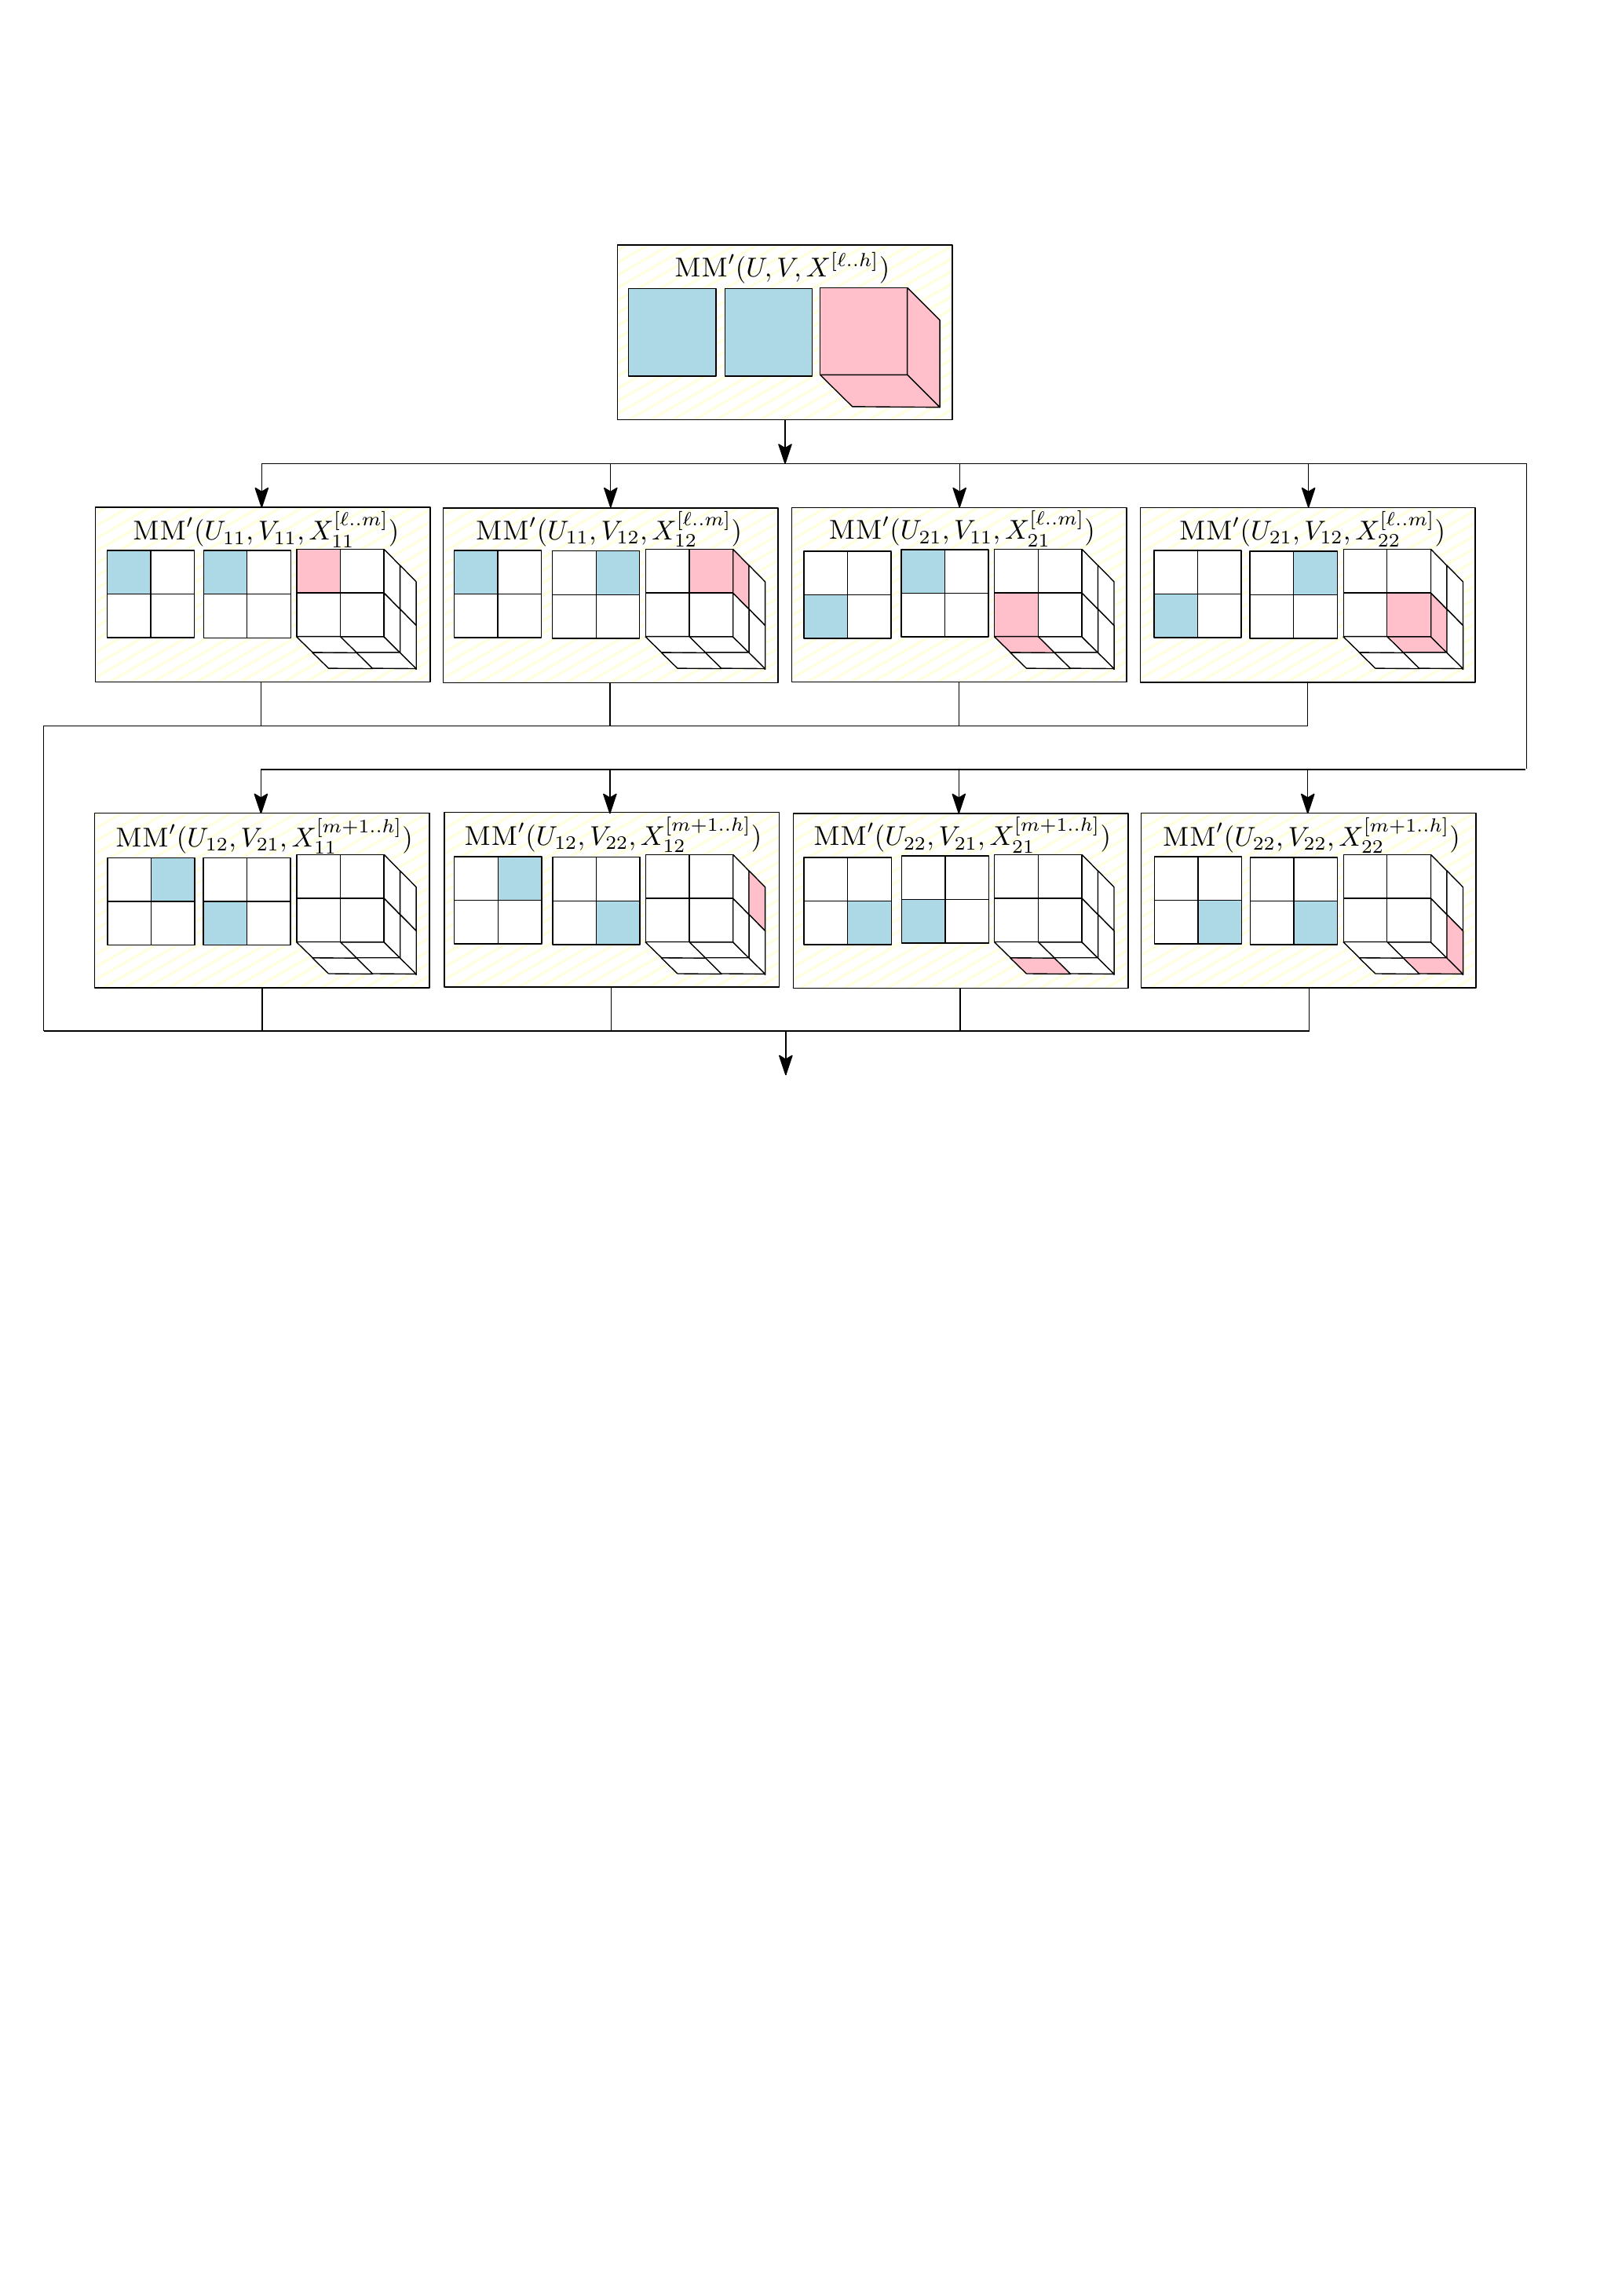}\\
\centering
\scalebox{0.7}{
\begin{tikzpicture}[thick,>=stealth',dot/.style = {draw,fill = blue,circle,inner sep = 0pt,minimum size = 4pt}]
  
\coordinate (O) at (0,0);
\draw[->] (-0.3,0) -- (6,0) coordinate[label = {below:Space}] (xmax);
\draw[->] (0,-0.3) -- (0,5) coordinate[label = {above:Span}] (ymax);

\node[dot,label={above:2-D}] (p1) at (1,4) {};
\node[dot,label={above:3-D}] (p2) at (5,1) {};
\node[dot,fill=red,label={above:2.5-D}] (pmid) at (2.5,2.87) {};
\node[label={left: {$n$}}] (p1left) at (0,4) {};
\node[label={left: {$\log n$}}] (p2left) at (0,1) {};
\node[label={left: {$n/r + \log n$}}] (pmidleft) at (0,2.87) {};
\node[label={below: {$n^2$}}] (p1down) at (1,0) {};
\node[label={below: {$n^3$}}] (p2down) at (5,0) {};
\node[label={below: {$rn^2$}}] (pmiddown) at (2.5,0) {};

\draw[dotted,color=blue] (p1) -- (pmid) -- (p2);
\draw[dotted,color=gray] (p1) -- (p1left);
\draw[dotted,color=gray] (p2) -- (p2left);
\draw[dotted,color=gray] (pmid) -- (pmidleft);
\draw[dotted,color=gray] (p1) -- (p1down);
\draw[dotted,color=gray] (p2) -- (p2down);
\draw[dotted,color=gray] (pmid) -- (pmiddown);
\end{tikzpicture}
}
\vspace{-0.3cm}
\end{minipage}
\caption{Top: Hybrid static 2.5-D algorithm's \textsc{MM-OPT$'$} function abbreviated as \textsc{MM$'$}. Bottom: Space-span trade-off for MM-OPT.}
\label{fig:mmhs-spacespan}
\vspace{-0.3cm}
\end{figure}

The space-span trade-off for \textsc{MM-OPT} is pictorially represented in Figure \ref{fig:mmhs-spacespan} (bottom). In the plot, the point denoted by 2.5-D need not be on the straight line joining points represented as 2-D and 3-D. We use a straight line for simplicity and pedagogical reasons.\\

\para{Processors vs. Space} It is important to note that we cannot improve the parallel running time of an MM algorithm consuming $\Th{n^3}$ space, but using a single processor only. Similarly, we cannot improve the parallel running time of the algorithm using $n^3$ processors, but consuming $\Th{n^2}$ space only (assuming no inter-processor communication). So, we might not be able to use all the processors and space available for the computation. We have the following lemma.

\begin{lemma}
Suppose we have $p$ processors in a shared-memory machine. Then, we can use at most $r$ planes to improve the parallel running time of the \textsc{MM-HD} and \textsc{MM-OPT} algorithms, where $(r-1)n^2 < p \le rn^2$ and $r \in [1, n]$.
\end{lemma}

\begin{figure*}
\centering
\begin{minipage}{0.46\textwidth}
\begin{mycolorbox}{$\textsc{TC\text{-}Loop}(X,U,V)$}
\begin{minipage}{0.99\textwidth}
{\codesize
\algotopspace{}
\noindent \scriptsize
\begin{enumerate}
\setlength{\itemindent}{-2em}
\vsitem \xparallelfor $i_1 \leftarrow 1$ \xto $n$ \xdo
\vsitem $\cdots$
\vsitem \xparallelfor $i_u \leftarrow 1$ \xto $n$ \xdo
\vsitem \T \xparallelfor $j_1 \leftarrow 1$ \xto $n$ \xdo
\vsitem \T $\cdots$
\vsitem \T \xparallelfor $j_v \leftarrow 1$ \xto $n$ \xdo
\vsitem \T \T $X[i_1,..,i_u,j_1,..,j_v] \gets 0$
\vsitem \T \T \xfor $k_1 \leftarrow 1$ \xto $n$ \xdo
\vsitem \T \T $\cdots$
\vsitem \T \T \xfor $k_x \leftarrow 1$ \xto $n$ \xdo
\vsitem \T \T \T $X[i_1,..,i_u,j_1,..,j_v] \gets X[i_1,..,i_u,j_1,..,j_v]$
\vsitem[] \T \T \T \T $+ U\{i_1,..,i_u,k_1,..,k_x\} \times V\{j_1,..,j_v,,k_1,..,k_x\}$
		
\algobottomspace{}
\end{enumerate}
}
\end{minipage}
\end{mycolorbox}
\vspace{-0.2cm}
\begin{mycolorbox}{$\textsc{TC}(X,U,V)$ \xcomment In-place}
\begin{minipage}{0.99\textwidth}
{\codesize
\algotopspace{}
\noindent \scriptsize
\begin{enumerate}
\setlength{\itemindent}{-2em}
\vsitem \xif $X,U,V$ are small tensors \xthen $\textsc{TC\text{-}Loop}(X,U,V)$
\vsitem \xelse
\vsitem \T \xparallelfor $i_1 \leftarrow 1$ \xto $2$ \xdo
\vsitem \T $\cdots$
\vsitem \T \xparallelfor $i_u \leftarrow 1$ \xto $2$ \xdo
\vsitem \T \T \xparallelfor $j_1 \leftarrow 1$ \xto $2$ \xdo
\vsitem \T \T $\cdots$
\vsitem \T \T \xparallelfor $j_v \leftarrow 1$ \xto $2$ \xdo
\vsitem \T \T \T \xfor $k_1 \leftarrow 1$ \xto $2$ \xdo
\vsitem \T \T \T $\cdots$
\vsitem \T \T \T \xfor $k_x \leftarrow 1$ \xto $2$ \xdo
\vsitem \T \T \T \T $\textsc{TC}(X_{i_1,..,i_u,j_1,..,j_v},U_{\{i_1,..,i_u,k_1,..,k_x\}},$
\vsitem[] \T \T \T \T \T \T $V_{\{j_1,..,j_v,k_1,..,k_x\}})$

\algobottomspace{}
\end{enumerate}
}
\end{minipage}
\end{mycolorbox}
\vspace{-0.2cm}
\begin{mycolorbox}{$\textsc{TC-HS}(X^{[0 .. r - 1]}, U, V)$ \xcomment Hybrid static}
\begin{minipage}{0.99\textwidth}
{\codesize
\vspace{-0.25cm}
\algorequire $\Th{r n^{u + v}}$ space, $r n^{u + v}$ processors

\noindent \scriptsize
\begin{enumerate}
\setlength{\itemindent}{-2em}

\vsitem Allocate $r \in [1, n^x]$ instances $X^{[0 .. r - 1]}$ of the tensor space
\vsitem \textsc{TC-HS$'$}$(X^{[0 .. r - 1]}, U, V)$ \xcomment $r = (2^x)^i, \text{where } i \in [1, \log n]$
\vsitem \textsc{TC-ReduceR}$(X^{[0..r - 1]}, n)$

\algobottomspace{}
\end{enumerate}
}
\end{minipage}
\end{mycolorbox}
\vspace{-0.2cm}
\begin{mycolorbox}{$\textsc{TC-HS}'(X^{[\ell..h]},U,V)$}
\begin{minipage}{0.99\textwidth}
{\codesize
\algotopspace{}
\noindent \scriptsize
\begin{enumerate}
\setlength{\itemindent}{-2em}

\vsitem \xif $\ell = h$ \xthen $\textsc{TC}(X^{[\ell]}, U, V)$ \xcomment Single instance
\vsitem \xelse \xcomment Multiple instances
%\vsitem \T $len \gets \ceil{ ( \ell + h ) / 2^{x} }$
\vsitem \T Split the range $[\ell, h]$ into $2^x$ partitions
\vsitem \T \xparallelfor $i_1 \leftarrow 1$ \xto $2$ \xdo
\vsitem \T $\cdots$
\vsitem \T \xparallelfor $i_u \leftarrow 1$ \xto $2$ \xdo
\vsitem \T \T \xparallelfor $j_1 \leftarrow 1$ \xto $2$ \xdo
\vsitem \T \T $\cdots$
\vsitem \T \T \xparallelfor $j_v \leftarrow 1$ \xto $2$ \xdo
\vsitem \T \T \T \xparallelfor $k_1 \leftarrow 1$ \xto $2$ \xdo
\vsitem \T \T \T $\cdots$
\vsitem \T \T \T \xparallelfor $k_x \leftarrow 1$ \xto $2$ \xdo
%\vsitem \T \T \T \T $div \gets \sum_{q = 1}^x (k_q - 1) \cdot 2^{x - q}$
%\vsitem \T \T \T \T $range \gets [len \cdot div \ldots \min(len \cdot (div + 1) - 1,$
%\vsitem[] \T \T \T \T \T $n - len \cdot (2^x - 1) )]$
\vsitem \T \T \T \T $p \gets \textsc{Linearize}(k_1, \ldots, k_x)$ \xcomment $p \in [1, 2^x]$
\vsitem \T \T \T \T $part \gets p$th partition 
\vsitem \T \T \T \T $\textsc{TC-HS}'(X_{i_1,..,i_u,j_1,..,j_v}^{part}$,
\vsitem[] \T \T \T \T \T $U_{\{i_1,..,i_u,k_1,..,k_x\}},V_{\{j_1,..,j_v,k_1,..,k_x\}})$

\algobottomspace{}
\end{enumerate}
}
\end{minipage}
\end{mycolorbox}
\end{minipage}
\begin{minipage}{0.53\textwidth}
\begin{mycolorbox}{$\textsc{TC-MM-OPT}(X,U,V)$}
\begin{minipage}{0.99\textwidth}
{\codesize

\algotopspace{}
\vspace{0.1cm}
\algorequire $x \ge 1$
\noindent \scriptsize
\begin{enumerate}
\setlength{\itemindent}{-2em}
\vsitem $\textsc{TT}(U',U, n, u+x)$ \xcomment{$U' \gets $ Transpose of tensor $U$}
\vsitem $\textsc{TT}(V',V, n, x+v)$ \xcomment{$V' \gets $ Transpose of tensor $V$}
\vsitem $\textsc{TF}(A,U', u, x)$ \xcomment{$A \gets $ Flatten tensor $U'$ to matrix}
\vsitem $\textsc{TF}(B,V', x, v)$
\xcomment{$B \gets $ Flatten tensor $V'$ to matrix}
\vsitem $\textsc{RMM-OPT}(C_{n^{u} \times n^{v}}, A_{n^{u} \times n^{x}}, B_{n^{x} \times n^{v}})$ \xcomment $C \gets A \times B$
\vsitem $\textsc{TD}(X, C, u, v)$
\xcomment{$X \gets$ Deflatten matrix $C$ to tensor}

\algobottomspace{}
\end{enumerate}
}
\end{minipage}
\end{mycolorbox}
\vspace{-0.2cm}
\begin{mycolorbox}{$\textsc{TT}(W,R,n,d)$ \xcomment Tensor Transposition}
\begin{minipage}{0.99\textwidth}
{\codesize

\algotopspace{}
\noindent \scriptsize
\begin{enumerate}
\setlength{\itemindent}{-2em}
\vsitem \xif $n = 1$ \xthen $W \gets R$
\vsitem \xelse
\vsitem \T $[r_1, \ldots, r_d] \gets$ rank vector
\vsitem[] \T (ranks of the indices of $R$ in the transposed tensor $W$) 
\vsitem \T \xparallelfor $p_1 \leftarrow 1$ \xto $2$ \xdo
\vsitem \T $\cdots$
\vsitem \T \xparallelfor $p_d \leftarrow 1$ \xto $2$ \xdo
\vsitem \T \T $\textsc{TT}(W_{p_1,..,p_d}, R_{p_{r_1},..,p_{r_d}}, n/2, d)$

\algobottomspace{}
\end{enumerate}
}
\end{minipage}
\end{mycolorbox}
\vspace{-0.2cm}
\begin{mycolorbox}{$\textsc{TF}(M,T,s', s'')$ \xcomment Tensor Flattening}
\begin{minipage}{0.99\textwidth}
{\codesize

\algotopspace{}
\noindent \scriptsize
\begin{enumerate}
\setlength{\itemindent}{-2em}
\vsitem \xif $n = 1$ \xthen $M \gets T$
\vsitem \xelse
\vsitem \T \xparallelfor $i_1 \leftarrow 1$ \xto $2$ \xdo
\vsitem \T $\cdots$
\vsitem \T \xparallelfor $i_{s'} \leftarrow 1$ \xto $2$ \xdo
\vsitem \T \T \xparallelfor $j_1 \leftarrow 1$ \xto $2$ \xdo
\vsitem \T \T $\cdots$
\vsitem \T \T \xparallelfor $j_{s''} \leftarrow 1$ \xto $2$ \xdo
\vsitem \T \T \T $I \gets \textsc{Linearize}(i_1, \ldots, i_{s'})$ \xcomment $I \in [1, 2^{s'}]$
\vsitem \T \T \T $J \gets \textsc{Linearize}(j_1, \ldots, j_{s''})$  \xcomment $J \in [1, 2^{s''}]$
\vsitem \T \T \T $\textsc{TF}(M_{I,J}, T_{i_1, ..,i_{s'},j_1,..,j_{s''}}, s', s'')$

\algobottomspace{}
\end{enumerate}
}
\end{minipage}
\end{mycolorbox}
\vspace{-0.2cm}
\begin{mycolorbox}{\textsc{RMM-OPT}$(X^{[0 .. r - 1]}_{a \times c}, U_{a \times b}, V_{b \times c})$ \xcomment Hybrid static 2.5-D}
\begin{minipage}{0.99\textwidth}
{\codesize
\vspace{-0.25cm}
\algorequire $\Th{rac}$ space, $rac$ processors

\noindent \scriptsize
\begin{enumerate}
\setlength{\itemindent}{-2em}

\vsitem Allocate $r \in [1, b]$ planes $X^{[0 .. r - 1]}$ all at once
\vsitem \textsc{RMM-OPT$'$}$(X^{[0 .. r - 1]}, U, V)$ \xcomment Uses $r \in [1, b]$ planes
\vsitem \textsc{MM-ReduceR}$(X^{[0..r - 1]}, a, c)$

\algobottomspace{}
\end{enumerate}
}
\end{minipage}
\end{mycolorbox}
\vspace{-0.2cm}
\begin{mycolorbox}{\textsc{RMM-OPT$'$}$(X^{[\ell .. h]}_{a \times c}, U_{a \times b}, V_{b \times c})$}
\begin{minipage}{0.99\textwidth}
{\codesize
\algotopspace{}
\noindent \scriptsize
\begin{enumerate}
\setlength{\itemindent}{-2em}

\vsitem \xif $\ell = h$ \xthen $\textsc{RMM}(X^{[\ell]}, U, V)$ \xcomment Single plane
\vsitem \xelse \xcomment Multiple planes

\vsitem \T \xif $a \ge \max(b, c)$ \xthen
\vsitem \T \T \xpar \textsc{RMM-OPT$'$}$(X_{T}^{[\ell .. h]}, U_{T}, V)$, \textsc{RMM-OPT$'$}$(X_{B}^{[\ell .. h]}, U_{B}, V)$ 
\vsitem \T \xelseif $b \ge \max(a, c)$ \xthen
\vsitem \T \T $m \gets (\ell + h) / 2$
\vsitem \T \T \xpar \textsc{RMM-OPT$'$}$(X^{[\ell .. m]}, U_{L}, V_{T})$, \textsc{RMM-OPT$'$}$(X^{[m+1 .. h]}, U_{R}, V_{B})$
\vsitem \T \xelseif $c \ge \max(a, b)$ \xthen
\vsitem \T \T \xpar \textsc{RMM-OPT$'$}$(X_{L}^{[\ell .. h]}, U, V_{L})$, \textsc{RMM-OPT$'$}$(X_{R}^{[\ell .. h]}, U, V_{R})$
\algobottomspace{}
\end{enumerate}
}
\end{minipage}
\end{mycolorbox}
\end{minipage}
\vspace{-0.4cm}
\caption{Algorithms for tensor contraction. \textsc{TC-Loop}: Iterative algorithm. \textsc{TC}: In-place recursive algorithm. \textsc{TC-HS}: Hybrid static algorithm. \textsc{TC-MM-OPT}: Hybrid static algorithm using MM.}
\label{fig:tensor-contraction}
\vspace{-0.2cm}
\end{figure*}

\para{\textsc{TC}: In-place Tensor Contraction Algorithm}
We now analyze the space-parallelism-locality trade-off for tensor contraction. An in-place recursive divide-and-conquer algorithm \textsc{TC} to solve the problem is presented in Figure \ref{fig:tensor-contraction}. The working of the \textsc{TC} algorithm from Figure \ref{fig:tensor-contraction} is similar to the working of the $\textsc{MM}$ algorithm from Figure \ref{fig:matrixmultiplication}. The matrices $U$, $V$, and $X$ are split along all dimensions into $2^{u + x}$, $2^{v + x}$, and $2^{u + v}$ orthants, respectively. As an example, $X_{1,2,1,2,2}$ is an orthant in 5 dimensions. The resulting tensor $X$ is computed using recursive divide-and-conquer on the orthants of $U$, $V$, and $X$. The function $\textsc{TC}(X, U, V)$ calls a total of $2^{u + v + x}$ number of child functions. There are $2^x$ number of parallel steps and in each parallel step $2^{u + v}$ number of child functions are run in parallel. A pictorial representation of the recursive \textsc{TC} algorithm using the fork-join model is shown in Figure \ref{fig:tensor-contraction-diagrams} (left). 

We analyze the complexity of $\textsc{TC}$ in the following lemma.

\begin{lemma}[\highlighttitle{TC: In-place}]
\label{lem:inplacetc}
The in-place TC algorithm has a complexity of $T_1(n) = \Th{n^{w}}$, $T_{\infty}(n)=\Th{n^{x} (u + v)}$, $Q_1(n) = \Oh{n^{w}/(BM^{(w/s)-1}) + n^{w}/M^{(w-s+1)/s} + n^s/B + n^{s - 1}}$, and $S_{\infty}(n) = \Th{n^{u + v}}$, where $w = u + v + x$ and $s = \max(u + x, v + x, u + v)$.
\end{lemma}
\begin{proof}
Total number of child functions of $\textsc{TC}$ is $2^{u + v + x} = 2^w$. Let the space occupied by all the three tensors $U$, $V$, and $X$ be $tspace = n^{u + x} + n^{v + x} + n^{u + v}$. Then, the recurrences for the complexities are:\\
\scalebox{0.8}
{
\centering
\begin{minipage}{0.49\textwidth}
\begin{align*}
& T_1(n) = T_{\infty}(n) = S_{\infty}(n) = \Th{1} \qquad \text{if } n = 1,\\
& T_1(n) = 2^w T_1(n / 2) + \Th{1} \qquad \text{if } n > 1.\\
& T_{\infty}(n) = 2^x ( T_{\infty}(n / 2) + \Th{u + v}) \qquad \text{if } n > 1.\\
& S_{\infty}(n) = 2^{u + v} S_{\infty}(n / 2) + \Th{1} \qquad \text{if } n > 1.\\
&Q_1(n) = \begin{cases} \Th{tspace/B + tspace/n} &\mbox{if } tspace \le \alpha M,\\ 
2^{w} Q_1(n / 2) + \Th{1}  & \mbox{if } tspace > \alpha M. \end{cases}
\end{align*}    
\end{minipage}
}\\

Recurrence for $T_{\infty}(n)$ is not straightforward. There are $2^x$ parallel steps. Each parallel step takes $T_{\infty}(n/2)$ parallel time for computing $2^{u + v}$ functions and $\Th{\log 2^{u + v}} = \Th{u + v}$ time for forking and joining (i.e., scheduling and syncing) $2^{u +  v}$ functions.
\vspace{-0.2cm}
\end{proof}

We could have theoretically improved the span to $T_{\infty}(n) = 2^x T_{\infty}(n / 2) + \Th{u + v}$ by eliminating all but one fork-join operation as shown in Figure \ref{fig:tensor-contraction-diagrams} (right). However, the current parallel schedulers that use the fork-join parallel computation model do not support this style of parallel computation.\\ 

\para{\textsc{TC-HS}: Hybrid Tensor Contraction} The \textsc{TC-HS} algorithm with static memory allocation is shown in Figure \ref{fig:tensor-contraction}. Let $|X| = n^{u + v}$ denote the number of elements in the output tensor $X$. Suppose $r|X|$ space and $r|X|$ processors are available. Then, we can use the available space and processors to improve the parallel running time
over that of the in-place \textsc{TC} algorithm.

\textsc{TC-HS} works as follows. Initially, we allocate space for $r$ tensors statically all at once before invoking \textsc{TC-HS$'$}, where $r$ is a power of $2^x$. \textsc{TC-HS$'$} calls itself $2^{u+v+x}$ times as there are $2^{u+v+x}$ orthants in the $(u+v+x)$-D computation space. Each of the $2^{u + v}$ orthants in the output tensor is updated by $2^x$ child functions. We make sure that the race condition never occurs by always having enough space ($\ge 2^x$ copies) for executing the child functions in parallel that write to the same orthant in the output.\\

\begin{theorem}[\highlighttitle{TC-HS: Hybrid Static}]
\label{thm:tc-hs}
\textsc{TC-HS} has a complexity of $T_1(n) = \Th{n^{w}}$, $T_{\infty}(n)=\Th{n^x(u + v)/r + (w\log r) / x}$, $Q_1(n) = \mathcal{O}(n^w/(BM^{(w/s)-1}) + n^w/M^{(w-s+1)/s}+ n^s r^{(w-s)/x} / B + n^{s-1}r^{(w-s+1)/x})$, and
$S_{\infty}(n) = \Th{r n^{u + v}}$.
\end{theorem}
\begin{proof} The recurrences are as follows:
\begin{center}
\scalebox{0.8}
{
\begin{minipage}{0.49\textwidth}
\begin{align*}
T_1(n, r) &= \begin{cases} \Th{n^w} &\mbox{if } r = 1, \\ 
2^w T_1(n/2, r/2) + \Th{1}  & \mbox{if } r > 1. \end{cases}\\
T_{\infty}(n, r) &= \begin{cases} \Th{n^x (u + v)} &\mbox{if } r = 1, \\ 
T_{\infty}(n/2, r/2) + \Th{u + v}  & \mbox{if } r > 1. \end{cases}\\
S_{\infty}(n, r) &\le \begin{cases} \Th{n^{u + v}} &\mbox{if } r = 1,\\
2^w S_{\infty}(n/2, r/2) + \Th{1}  & \mbox{if } r > 1. \end{cases}\\
Q_1(n, r) &= \begin{cases} \Oh{n^w / (BM^{(w/s) - 1}) +n^{w}/M^{(w-s+1)/s} + n^s/B + n^{s - 1}} &\mbox{if } r = 1, \\ 
2^w Q_1(n/2, r/2) + \Oh{1}  & \mbox{if } r > 1. \end{cases}
\end{align*}
\end{minipage}
}
\end{center}
\end{proof}

\begin{lemma}[\highlighttitle{Reordering TC loops}]
\label{lem:reordertc}
The $i$, $j$, $k$ loops of \textsc{TC-Loop} can be reordered in $w!$ ways without affecting correctness. 
\end{lemma}
\begin{proof}
Consider the cell $X[i_1 = i_1', \ldots ,i_u = i_u',j_1 = j_1', \ldots ,j_v \allowbreak = j_v']$ in the resulting tensor $X$. This cell does not depend directly or indirectly on any other cell $X[i_1'+\Delta i_1', \ldots ,i_u' + \Delta i_u', j_1' + \Delta j_1', \ldots , j_v' + \Delta j_v']$ for all feasible values of $\Delta i_1', \ldots, \allowbreak \Delta i_u', \allowbreak \Delta j_1', \ldots, \Delta j_v'$ such that at least one of them is non-zero. Hence, we can reorder the $u + v$ number of $i$ and $j$ loops without affecting correctness. 

The $k$-loops cannot be parallelized without using reduction because parallelizing them will lead to race conditions. The total number of computations required to update the cell $X[i_1', \ldots ,i_u',j_1', \ldots ,j_v']$ is $n^x$, which is obtained from the dot product of $x$-D computation hypercubes that are present in $U$ and $V$, analogous to the dot product of vectors for matrix multiplication. If the addition operator is both commutative and associative (e.g.: $+$ in our problem), it does not matter in which (sequential) order we perform $n^x$ computations. Hence, we can order $k$-loops in any way among themselves and also interspersing the $k$-loops with the $i$- and $j$-loops leading to a total of $(u + v + x)!$ orderings without affecting correctness. 
\end{proof}

\noindent
\highlighttitle{TC-HS: Hybrid static 2.5-D}.

\begin{align*} 
&Q_1(n,r) = 2^w Q_1\Big(\frac{n}{2}, \frac{r}{2^x}\Big) + \frac{n^s}{B}+n^{s-1} \\
    &=2^w\Big( 2^w Q_1\bigg(\frac{n}{2^2}, \frac{r}{(2^x)^2}\bigg) + \frac{1}{B}\bigg(\frac{n}{2}\bigg)^s + \bigg(\frac{n}{2}\bigg)^{s-1} \Big) + \frac{n^s}{B}+n^{s-1} \\
    &= 2^{2w}Q_1\bigg(\frac{n}{2^2}, \frac{r}{(2^x)^2}\bigg)+ \frac{1}{B}n^s 2^{w-s} +n^{s-1}2^{w-s+1}+ \frac{n^s}{B}+n^{s-1}\\
    &=2^{\frac{w\log r}{x}}Q_1\bigg(\frac{n}{2^{(\log r)/x}}, \frac{r}{(2^x)^{\log r/x}}\bigg) \\
    & \quad +\frac{1}{B}n^s 2^{(\frac{\log r}{x}-1)(w-s)} +n^{s-1}2^{(\frac{\log r}{x}-1)(w-s+1)} \\
 &= r^{w/x}\Bigg(\frac{(n/r^{1/x})^w}{BM^{(w/s)-1}} + \frac{(n/r^{1/x})^w}{M^{(w-s+1)/s}}+\frac{(n/r^{1/x})^s}{B} + (n/r^{1/x})^{s-1}\Bigg)\\
 &\quad +  \frac{1}{B}n^s 2^{(\frac{\log r}{x}-1)(w-s)} +n^{s-1}2^{(\frac{\log r}{x}-1)(w-s+1)} \\
 &= O\Bigg(\frac{n^w}{BM^{(w/s)-1}} + \frac{n^w}{M^{(w-s+1)/s}}+ \frac{1}{B}n^s 2^{(\frac{\log r}{x})(w-s)} +n^{s-1}2^{(\frac{\log r}{x})(w-s+1)}\Bigg) \\
 &=O\Bigg(\frac{n^w}{BM^{(w/s)-1}} + \frac{n^w}{M^{(w-s+1)/s}}+ \frac{1}{B}n^s r^{(w-s)/x} + n^{s-1}r^{(w-s+1)/x}\Bigg).
\end{align*}

\begin{align*}
&T_{\infty}(n,r) = T_{\infty}\left( \frac{n}{2},\frac{r}{2^x} \right) + w = T_{\infty}\left( \frac{n}{2^i},\frac{r}{(2^x)^i} \right) + iw\\
&= \Th{ \left( \frac{n}{2^{(\log r) / x}} \right)^x (u + v) } + \frac{w \log r}{x} \qquad \left( r = (2^x)^i \right)\\
&= \frac{n^x (u + v)}{r} + \frac{w \log r }{x}
\end{align*}

\begin{lemma}[\highlighttitle{RMM-OPT}]
\label{thm:rMM-OPT}
\textsc{RMM-OPT} has a complexity of $T_{\infty}(a,b,c,r)=\Th{b/r + \log (rac)}$ and $Q_1(a, b, c, r) = (rac / (a'c')) \times Q_{1}'(a', b', c', 1)$, where $b' = b/r, a' = \min (a, b'),$ and $c' = \min (c, b')$ and $Q_{1}'(a', b', c', 1) = \Oh{a'b'c'/(B \sqrt{M}) + a'b'c'/M + (a'b'+b'c'+c'a')/B + (a'+b'+c')}$.
\end{lemma}
\begin{proof} We assume that $a, b, $ and $c$ are powers of 2 for simplicity. Let $T_{\infty}'(a, b, c, r)$ and $N_{\infty}(a, b, c, r)$  represent the span and the number of supersteps in the span for \textsc{RMM-OPT}$'$, respectively. Then\\
\scalebox{0.9}
{
\centering
\begin{minipage}{0.49\textwidth}
\begin{align*}
&N_{\infty}(a, b, c, r) = \begin{cases} 
\left.
\begin{cases}
1 & \mbox{if } a = b = c = 1,\\
N_{\infty}(a/2, b, c) + 1 & \mbox{if } a \ge \max(b, c),\\
2 N_{\infty}(a, b/2, c) + 1  & \mbox{if } b \ge \max(a, c),\\
N_{\infty}(a, b, c/2) + 1  & \mbox{if } c \ge \max(a, b).
\end{cases}
\right\}
&\mbox{if } r = 1,\\
\left.
\begin{cases}
N_{\infty}(a/2, b, c, r) + 1  & \mbox{if } a \ge \max(b, c),\\
N_{\infty}(a, b/2, c, r/2) + 1  & \mbox{if } b > \max(a, c),\\
N_{\infty}(a, b, c/2, r) + 1  & \mbox{if } c \ge \max(a, b).
\end{cases}
\right\}
&\mbox{if } r > 1.
\end{cases} 
\end{align*}    
\end{minipage}
}\\

\noindent
\textit{Base case.} At the base case $(r = 1)$, we use only one plane to perform rectangular MM using the recursive algorithm from \cite{FrigoLePrRa1999}. It takes $\log a$ (resp. $\log c$) steps for $a$ (resp. $c$) to reduce to 1. Similarly, it takes $2^{\log b} = b$ steps for $b$ to reduce to 1. Hence, in total, $N_{\infty}(a, b, c, 1) = b + \log a + \log c = b + \log (ac)$. 

\vspace{0.1cm}
\noindent
\textit{Recursion case.} To use the base case, we need to compute the possibly decreased values of $a, b,$ and $c$ when $r$ reaches $1$. Three cases arise:\\
$[$Case 1. Compute the final value of $b.]$ In this case, the total number of parallel steps required to reach the base case is $\log r$ because $b$ will be decreased the same number of times as that of $r$. So, the final value of $b$ at the base case will be $b/r$.\\
$[$Case 2. Compute the final value of $a.]$ The final value of $a$ at the base case will be $\min (a, b/r)$ from the following two subcases:\\
$($Subcase $(i).$ $a$ decreases at least once.$)$ This subcase happens when $r \ge b/a$. When $b$ value decreases to a point such that it is the same as $a$, then both the values decrease by a factor of 2 in a fixed constant number of parallel time steps. Hence, the decreased value of $a$ will be $b/r$. $($Subcase $(ii).$ $a$ never decreases.$)$ This subcase happens when $r < b/a$. In this case, the value of $r$ decreases to 1 before $b$ reaches the value of $a$. Hence, the final value of $a$ at the base case is unchanged and will be $a$.\\
$[$Case 3. Compute the final value of $c.]$ Using the logic from Case 2, the final value of $c$ at the base case can be computed to be $\min (c, b/r)$.

Using the final values of $a,b,$ and $c$ at the base case, we can now compute $N_{\infty}(a, b, c, r)$. The number of times $b$ will be decreased until it reaches the base case is $\log r$. The number of times $a$ will be decreased is $\log (a/(\text{final value of a}) = \log (a/\min(a, b/r)) =$\\$\max(0, \log (ar/b))$. Similarly, the number of times $c$ will be decreased until base case is $\log (c/\min(c, b/r)) = \max(0, \log (cr/b))$. 

Let $b' = b/r, a' = \min (a, b'),$ and $c' = \min (c, b')$. We have\\
\scalebox{1}
{
\centering
\begin{minipage}{0.49\textwidth}
\begin{align*}
N_{\infty}(a,b,c,r) &= N_{\infty} \text{ for recursion} + N_{\infty} \text{ for base case}\\
&= [\log r + \log (a / a') + \log (c / c')] +  N_{\infty}(a', b', c', 1)\\
&= [\log (rac / (a'c'))] + [b' + \log (a'c' )]\\
&= b/r + \log (rac)\\
T_{\infty}'(a,b,c,r) &= \Th{N_{\infty}(a,b,c,r)} = \Th{b/r + \log (rac)}
\end{align*}    
\end{minipage}
}\\

The serial cache complexity for \textsc{RMM-OPT}$'$ is\\
\scalebox{0.8}
{
\centering
\begin{minipage}{0.49\textwidth}
\begin{align*}
&Q_{1}'(a, b, c, r) = \begin{cases} 
\Oh{abc/(B \sqrt{M}) + abc/M + (ab+bc+ca)/B + (a+b+c)}
&\mbox{if } r = 1,\\
\left.
\begin{cases}
2Q_{1}'(a/2, b, c, r) + \Th{1}  & \mbox{if } a \ge \max(b, c),\\
2Q_{1}'(a, b/2, c, r/2) + \Th{1}  & \mbox{if } b > \max(a, c),\\
2Q_{1}'(a, b, c/2, r) + \Th{1}  & \mbox{if } c \ge \max(a, b).
\end{cases}
\right\}
&\mbox{if } r > 1.
\end{cases} 
\end{align*}    
\end{minipage}
}\\

The complexity of $Q_{1}'(a, b, c, 1)$ at the base case is taken from \cite{FrigoLePrRa1999}. Note that at any level of the recursion tree, the values of the ordered tuple $(a, b, c)$ will be the same for all function calls at that level. This means that\\
\scalebox{1}
{
\centering
\begin{minipage}{0.49\textwidth}
\begin{align*}
Q_{1}'(a,b,c,r) &= \text{Number of leaf nodes} \times Q_{\infty}' \text{ for a leaf node}\\
&= 2^{N_{\infty} \text{ for recursion}} \times Q_{1}'(a', b', c', 1)\\
&= 2^{\log (rac / (a'c'))} \times Q_{1}'(a', b', c', 1)\\
&= (rac / (a'c')) \times Q_{1}'(a', b', c', 1)
\end{align*}    
\end{minipage}
}\\

$T_{\infty}''(n)$ and $Q_{1}''(n)$ for \textsc{MM-ReduceR} are $\Th{\log n + B}$ and \\
$\Th{rac/B + r (a + c)}$, respectively. So, solving the equations $T_{\infty}=T_{\infty}' + T_{\infty}''$ and $Q_{1}=Q_{1}' + Q_{1}''$, we get the lemma.
\end{proof}

\begin{theorem}[\highlighttitle{TC-MM-OPT: TC with Hybrid Static MM}]
\label{thm:tc-MM-OPT}
\textsc{TC-MM-OPT} has a complexity of $T_{\infty}(n)=\Th{n^x/r + w \log n + \log r}$ and $Q_1(n) = Q_{1}^{RMM-OPT}(n^u, n^x, n^v, r)$.
\end{theorem}
\begin{proof} The recurrences for \textsc{TT} and \textsc{TF} are:\\
\scalebox{0.8}
{
\centering
\begin{minipage}{0.49\textwidth}
\begin{align*}
& T_{\infty}^{TT}(n) = T_{\infty}^{TF}(n) = \Th{1} \qquad \text{if } n = 1,\\
%& T_1^{TT}(n) = 2^d T_1^{TT}(n / 2) + \Th{1} \qquad \text{if } n > 1.\\
& T_{\infty}^{TT}(n) = T_{\infty}^{TT}(n / 2) + \Th{d} \qquad \text{if } n > 1.\\
& T_{\infty}^{TF}(n) = T_{\infty}^{TF}(n / 2) + \Th{s' + s''} \qquad \text{if } n > 1.\\
%& S_{\infty}^{TT}(n) = 2^{d} S_{\infty}^{TT}(n / 2) + \Th{1} \qquad \text{if } n > 1.\\
&Q_1^{TT}(n) = \begin{cases} \Th{n^d/B + n^{d-1}} &\mbox{if } n^d \le \alpha M,\\ 
2^{d} Q_1^{TT}(n / 2) + \Th{1}  & \mbox{if } n^d > \alpha M. \end{cases}\\
&Q_1^{TF}(n) = \begin{cases} \Th{n^{(s' + s'')}/B + n^{(s' + s'' - 1)}} &\mbox{if } n^{s' + s''} \le \alpha M,\\ 
2^{s' + s''} Q_1^{TF}(n / 2) + \Th{1}  & \mbox{if } n^{s' + s''} > \alpha M. \end{cases}
\end{align*}    
\end{minipage}
}\\

Solving the recurrences, we get $T_{\infty}^{TT}(n) = \Th{d \log n}$, $T_{\infty}^{TF}(n) = \Th{(s' + s'') \log n}$, $Q_{1}^{TT}(n) = \Th{n^d/B + n^d/M^{1/d} + n^{d-1}}$, and\\
$Q_{1}^{TF}(n) = \Th{n^{s' + s''}/B + n^{s' + s''}/M^{1/(s' + s'')} + n^{s' + s''-1}}$.

\hide{
\scalebox{0.8}
{
\centering
\begin{minipage}{0.49\textwidth}
\begin{align*}
& T_1^{TF}(n) = T_{\infty}^{TF}(n) = S_{\infty}^{TF}(n) = \Th{1} \qquad \text{if } n = 1,\\
& T_1^{TF}(n) = 2^{(s + s')} T_1^{TF}(n / 2) + \Th{1} \qquad \text{if } n > 1.\\
& T_{\infty}^{TF}(n) = T_{\infty}^{TF}(n / 2) + \Th{s + s'} \qquad \text{if } n > 1.\\
& S_{\infty}^{TF}(n) = 2^{(s + s')} S_{\infty}^{TF}(n / 2) + \Th{1} \qquad \text{if } n > 1.\\
&Q_1^{TF}(n) = \begin{cases} \Th{n^{(s + s')}/B + n^{(s + s' - 1)}} &\mbox{if } n^{s + s'} \le \alpha M,\\ 
2^{s + s'} Q_1^{TF}(n / 2) + \Th{1}  & \mbox{if } n^{s + s'} > \alpha M. \end{cases}
\end{align*}    
\end{minipage}
}\\
}

The complexity for \textsc{TC-MM-OPT} is:\\
\scalebox{0.8}
{
\centering
\begin{minipage}{0.49\textwidth}
\begin{align*}
 T_{\infty} &= T_{\infty}^{TT}(U' \gets U) + T_{\infty}^{TT}(V' \gets V) + T_{\infty}^{TF}(A \gets U') +\\
&\qquad T_{\infty}^{TF}(B \gets V') +
T_{\infty}^{RMM-OPT}(C \gets A \times B) + T_{\infty}^{TD}(X \gets C)\\
&= \Th{n^x/r + w \log n + \log r}\\
 Q_{1} &= Q_{1}^{TT}(U' \gets U) + Q_{1}^{TT}(V' \gets V) + Q_{1}^{TF}(A \gets U') +\\
&\qquad Q_{1}^{TF}(B \gets V') +
Q_{1}^{RMM-OPT}(C \gets A \times B) + Q_{1}^{TD}(X \gets C)\\
&= Q_{1}^{RMM-OPT}(n^u, n^x, n^v, r)
\end{align*}    
\end{minipage}
}\\

\end{proof}
